# Supplementary material for: Routing-Free Mixture-of-Experts
Source: arXiv:2604.00801 source file (2026-04-01)
Supplement: Supplementary file 1 [file _appendix.tex]

\newpage
\section*{Appendix}

\begin{table}[t]
\centering
\scriptsize
\addtolength{\tabcolsep}{-2.5pt} 
\begin{tabular}{l|ll|ccc|cccc|cccc}
\toprule
    & \multicolumn{2}{c|}{\textbf{Learning Style}} 
    & \multicolumn{3}{c|}{\textbf{\#Parameters}} 
    & \multicolumn{4}{c|}{\textbf{Image Question Answering}} 
    & \multicolumn{2}{c}{\textbf{Benchmark}} \\
    LLM Backbone  & Adapter & Architecture 
    & Act. & Tr. & Total
    & VisWiz$^\text{D}$ & VisWiz$^\text{S}$    
    & SQA$^\text{I}$    & VQA$^\text{T}$
    & MMB               & LLaVA$^\text{W}$    \\    
\midrule
    Mixtral-8$\times$7B 
    & LoRA$_{32}$  & Attention
    & 13B &  M & 47B
    &       & 
    &       & \\
    Mixtral-8$\times$7B 
    & LoRA$_{128}$ & Attention
    & 13B &  M & 47B
    &       & 
    &       & \\
\midrule
\rowcolor{LightRed}
    Mixtral-8$\times$7B 
    & LoRA$_{32}$ & \modelname{} $\times4$-Top1
    & 13B & M & 47B
    &       & 
    &       & \\
\rowcolor{LightRed}
    Mixtral-8$\times$7B 
    & PA$_{32}$ & \modelname{} $\times4$-Top1
    & 13B & M & 47B
    &       & 
    & 54.3  & \\
\rowcolor{LightRed}
    Mixtral-8$\times$7B 
    & LoRA$_{16}$ & \modelname{} $\times8$-Top2
    & 13B & M & 47B
    &       & 
    &       & \\
\rowcolor{LightRed}
    Mixtral-8$\times$7B 
    & PA$_{16}$ & \modelname{} $\times8$-Top2
    & 13B & M & 47B
    &       & 
    &       & \\
\rowcolor{LightRed}
    Mixtral-8$\times$7B 
    & LoRA$_{16}$ & \modelname{}-E $\times8$-Top2
    & 13B & M & 47B
    &       & 
    &       & \\
\rowcolor{LightRed}
    Mixtral-8$\times$7B 
    & PA$_{16}$ & \modelname{}-E $\times8$-Top2      
    & 13B & M & 47B
    &       & 
    &       & \\
\rowcolor{LightRed}
    Mixtral-8$\times$7B 
    & LoRA$_{32}$ & \modelname{}-D $\times4$
    & 13B & M & 47B
    & 51.1  & 50.8
    & 65.6  & \\
\rowcolor{LightRed}
    Mixtral-8$\times$7B 
    & PA$_{32}$ & \modelname{}-D $\times4$
    & 13B & M & 47B
    &       & 
    &       & \\
\rowcolor{LightRed}
    Mixtral-8$\times$7B 
    & LoRA$_{32}$   & \modelname{}-S
    & 13B & M & 47B
    &       & 
    & 57.6  & \\
\rowcolor{LightRed}
    Mixtral-8$\times$7B 
    & PA$_{32}$ & \modelname{}-S
    & 13B & M & 47B
    & 55.9  & 
    & 58.1  & \\
\bottomrule
\end{tabular}
\caption{\textbf{Evaluation results for baseline methods and \modelname{} variants trained with complete LLaVA-1.5 pretraining data and 20\% of instruction fine-tuning data.} ``Act.'', ``Tr.'', ``PT'' and ``IT'' respectively denote the number of activated parameters, trainable parameters, pretraining samples and instruction tuning samples. Evaluation benchmark names are abbreviated, including VisWiz$^\text{D}$ \& VisWiz$^\text{S}$: the dev and standard partitions of VizWiz-VQA \citep{gurari2018vizwiz}; SQA$^\text{I}$: ScienceQA-IMG \citep{lu2022scienceqa}; VQA$^\text{T}$: TextVQA \citep{singh2019textvqa}; MMB: MMBench \citep{liu2023mmbench}; LLaVA$^\text{W}$: LLaVA-Bench (In-the-Wild) \citep{liu2024llava}. ``PA'' indicates parallel adapter.}
\label{tab:result20}
\end{table}

\begin{table}[t]
\centering
\scriptsize
\addtolength{\tabcolsep}{-3pt} 
\begin{tabular}{l|ll|ccc|cc|cccc|cccc}
\toprule
    & \multicolumn{2}{c|}{\textbf{Learning Style}} 
    & \multicolumn{3}{c|}{\textbf{\#Parameters}} 
    & \multicolumn{2}{c|}{\textbf{\#Samples}} 
    & \multicolumn{4}{c|}{\textbf{Image Question Answering}} 
    & \multicolumn{2}{c}{\textbf{Benchmark}} \\
    LLM Backbone  & Adapter & Architecture 
    & Act. & Tr. & Total
    & PT   & IT  
    & VisWiz$^\text{D}$ & VisWiz$^\text{S}$    
    & SQA$^\text{I}$    & VQA$^\text{T}$
    & MMB               & LLaVA$^\text{W}$    \\    
\midrule   
    Vicuna-7B     & \multicolumn{2}{c|}{Full fine-tuning}
    & 6.7B & 6.7B & 6.7B
    & 558K  & 665K  
    & ---   & 50.0  
    & 66.8  & 58.2
    & 64.3  & 58.3 \\
    Vicuna-13B    & \multicolumn{2}{c|}{Full fine-tuning}
    & 13B & 13B & 13B
    & 558K  & 665K  
    & ---   & 53.6  
    & 71.6  & 61.3
    & 67.7  & 63.6 \\
\midrule  
    StableLM-1.6B & \multicolumn{2}{c|}{Full fine-tuning + MoE-fy}
    & 2.0B & 2.9B & 2.9B
    & 558K  & 1.6M
    & ---   & 37.2
    & 62.6  & 47.8
    & 59.4  & 85.9 \\
    Qwen-1.8B     & \multicolumn{2}{c|}{Full fine-tuning + MoE-fy}
    & 2.2B & 3.1B & 3.1B
    & 558K  & 1.6M  
    & ---   & 32.3  
    & 63.1  & 48.0
    & 59.7  & 88.7 \\
    Phi-2-2.7B    & \multicolumn{2}{c|}{Full fine-tuning + MoE-fy}
    & 3.6B & 5.3B & 5.3B
    & 558K  & 1.6M  
    & ---   & 43.4  
    & 68.7  & 50.2
    & 65.5  & 93.2 \\
\midrule
    Mixtral-8$\times$7B 
    & LoRA$_{32}$  & Attention
    & 13B &  M & 47B
    & 558K  & 665K  
    & 39.7  & 
    & 70.4  & \\
    Mixtral-8$\times$7B 
    & LoRA$_{128}$ & Attention
    & 13B &  M & 47B
    & 558K  & 665K  
    & 52.8  & 52.9  
    & 71.0  & \\
\midrule
\rowcolor{LightRed}
    Mixtral-8$\times$7B 
    & LoRA$_{32}$ & \modelname{} $\times4$-Top1
    & 13B & M & 47B
    & 558K  & 665K  
    &       & 
    & 58.7  & \\
\rowcolor{LightRed}
    Mixtral-8$\times$7B 
    & PA$_{32}$ & \modelname{} $\times4$-Top1
    & 13B & M & 47B
    & 558K  & 665K  
    &       & 
    &       & \\
\rowcolor{LightRed}
    Mixtral-8$\times$7B 
    & LoRA$_{16}$ & \modelname{} $\times8$-Top2
    & 13B & M & 47B
    & 558K  & 665K  
    &       & 
    &       & \\
\bottomrule
\end{tabular}
\caption{\textbf{Evaluation results of baseline methods and \modelname{} variants trained with complete LLaVA-1.5 pretraining and instruction fine-tuning data.} }
\label{tab:inference_cost}
\end{table}
